# Supplementary material for: Learning Task Skills and Goals Simultaneously from Physical Interaction
Source: arXiv:2309.04596 source file (2023-09-08)
Supplement: Supplementary file 1 [file Appendix.tex]

\section{Appendix}
\label{sec:append}
Not provided in the submitted version
